# Supplementary material for: Combined Flicker-banding and Moire Removal for Screen-Captured Images
Source: arXiv:2602.01559 source file (2026-02-02)
Supplement: Supplementary file 1 [file supp.tex]

%%%%%%%% ICML 2026 EXAMPLE LATEX SUBMISSION FILE %%%%%%%%%%%%%%%%%

\documentclass{article}

% Recommended, but optional, packages for figures and better typesetting:
\usepackage{microtype}
\usepackage{graphicx}
\usepackage{subcaption}
\usepackage{booktabs} % for professional tables

% hyperref makes hyperlinks in the resulting PDF.
% If your build breaks (sometimes temporarily if a hyperlink spans a page)
% please comment out the following usepackage line and replace
% \usepackage{icml2026} with \usepackage[nohyperref]{icml2026} above.
\usepackage{hyperref}

% Attempt to make hyperref and algorithmic work together better:

% Use the following line for the initial blind version submitted for review:
\usepackage{icml2026}

% For preprint, use
% \usepackage[preprint]{icml2026}

% If accepted, instead use the following line for the camera-ready submission:
% \usepackage[accepted]{icml2026}

\usepackage{amsmath}
\usepackage{amssymb}
\usepackage{mathtools}
\usepackage{amsthm}

% if you use cleveref..
\usepackage[capitalize,noabbrev]{cleveref}

%%%%%%%%%%%%%%%%%%%%%%%%%%%%%%%%
% THEOREMS
%%%%%%%%%%%%%%%%%%%%%%%%%%%%%%%%
\theoremstyle{plain}

\theoremstyle{definition}

\theoremstyle{remark}

\usepackage{xcolor}
\usepackage{colortbl}
\usepackage{booktabs}
% Todonotes is useful during development; simply uncomment the next line
%    and comment out the line below the next line to turn off comments
%\usepackage[disable,textsize=tiny]{todonotes}
\usepackage[textsize=tiny]{todonotes}

% The \icmltitle you define below is probably too long as a header.
% Therefore, a short form for the running title is supplied here:
\icmltitlerunning{Combined Flicker-banding and Moire Removal for Screen-Captured Images: Supplementary Material}

\begin{document}

\twocolumn[
  \icmltitle{Combined Flicker-banding and Moiré Removal \\ for Screen-Captured Images: Supplementary Material}

  % It is OKAY to include author information, even for blind submissions: the
  % style file will automatically remove it for you unless you've provided
  % the [accepted] option to the icml2026 package.

  % List of affiliations: The first argument should be a (short) identifier you
  % will use later to specify author affiliations Academic affiliations
  % should list Department, University, City, Region, Country Industry
  % affiliations should list Company, City, Region, Country

  % You can specify symbols, otherwise they are numbered in order. Ideally, you
  % should not use this facility. Affiliations will be numbered in order of
  % appearance and this is the preferred way.
  
  \icmlsetsymbol{equal}{*}

   \begin{icmlauthorlist}
    \icmlauthor{Firstname1 Lastname1}{equal,yyy}
    \icmlauthor{Firstname2 Lastname2}{equal,yyy,comp}
    \icmlauthor{Firstname3 Lastname3}{comp}
    \icmlauthor{Firstname4 Lastname4}{sch}
    \icmlauthor{Firstname5 Lastname5}{yyy}
    \icmlauthor{Firstname6 Lastname6}{sch,yyy,comp}
    \icmlauthor{Firstname7 Lastname7}{comp}
    %\icmlauthor{}{sch}
    \icmlauthor{Firstname8 Lastname8}{sch}
    \icmlauthor{Firstname8 Lastname8}{yyy,comp}
    %\icmlauthor{}{sch}
    %\icmlauthor{}{sch}
  \end{icmlauthorlist}

  \icmlaffiliation{yyy}{Department of XXX, University of YYY, Location, Country}
  \icmlaffiliation{comp}{Company Name, Location, Country}
  \icmlaffiliation{sch}{School of ZZZ, Institute of WWW, Location, Country}

  \icmlcorrespondingauthor{Firstname1 Lastname1}{first1.last1@xxx.edu}
  \icmlcorrespondingauthor{Firstname2 Lastname2}{first2.last2@www.uk}

  % You may provide any keywords that you find helpful for describing your
  % paper; these are used to populate the "keywords" metadata in the PDF but
  % will not be shown in the document
  \icmlkeywords{Machine Learning, ICML}

  \vskip 0.3in
]

% this must go after the closing bracket ] following \twocolumn[ ...

% This command actually creates the footnote in the first column listing the
% affiliations and the copyright notice. The command takes one argument, which
% is text to display at the start of the footnote. The \icmlEqualContribution
% command is standard text for equal contribution. Remove it (just {}) if you
% do not need this facility.

% Use ONE of the following lines. DO NOT remove the command.
% If you have no special notice, KEEP empty braces:

\printAffiliationsAndNotice{}  % no special notice (required even if empty)
% Or, if applicable, use the standard equal contribution text:
% \printAffiliationsAndNotice{\icmlEqualContribution}
\suppressfloats
\begin{figure*}[t!]
    \centering
    \includegraphics[width=\textwidth]{figures/supp_moire.pdf}
    \caption{Example of moiréing patterns, such as mesh patterns, ripple patterns, color splotches etc.}
    \label{fig:examplemoire}
\end{figure*}
\suppressfloats
\begin{figure*}[t!]
    \centering
    \includegraphics[width=\textwidth]{figures/supp_banding.png}
    \caption{Example of banding patterns, such as jagged bands, striped flickering etc.}
    \label{fig:examplebanding}
\end{figure*}
\section{Formation Mechanism}
\subsection{Formation Mechanism of Moiréing}
Moiréing artifacts result from the superposition of two or more periodic structures with similar spatial frequencies~\cite{Sun_2018}. This pattern occurs even when these similar structures overlap with each other with only a slight offset and the bigger the offset, the more obvious the moiréing patterns are. Moiréing patterns have various shapes, such as stripes, circles and so on~\cite{Dual_domain}. Even though the moiréing artifact is an optical phenomenon, this pattern is significant in the computer field.

Similar to the optical formation of moiréing artifacts, the digital moiréing artifacts appear when taking photos on the screen. This digital pattern results from the interference between two overlapping pixel matrices~\cite{hefhde2net}: the pixel grids of the display screens and the pixel grids of the cameras. When smartphone cameras take photos, the periodic pixel structure of the display screens interacts with that of the cameras. If these two kinds of grids don't match each other properly, due to the slight difference of camera angles, distance and frequency, moiréing artifacts appear.

In the frequency domain, moiréing artifacts usually cross a wide range of frequency and exhibit non-uniform and anisotropic spatial distribution. Different from common image noise, moiréing patterns don't distribute randomly but present structural characteristics and are often accompanied by color distortion~\cite{dai2022video}. Due to the interaction between two structures, moiréing artifacts have an obvious local variation characteristic that within the same image, certain regions may appear as high-frequency, fine stripes, while other regions may show low-frequency, broad ripples. Some examples of moiréing artifacts in different shapes are shown in the Figure~\ref{fig:examplemoire} below.

%%So image demoiréing becomes a challenging image restoration task because traditional methods designed to remove single pattern are often ineffective in handling such composite artifacts~\cite{Chengmulti2019}.  

\subsection{Formation Mechanism of Flicker-banding}
Flicker-banding shows as light and dark stripes in the photos, such as cracked banding, striped flickering, grid-like artifacts, curve banding and so on. When taking pictures, you may find an interesting fact that the shorter the exposure time is, the darker the stripes are. Changing the exposure time, you may get some different banding. There are some examples of flicker-banding in different shapes shown in the Figure~\ref{fig:examplebanding} below. Flicker-banding appears due to the temporal inconsistency between cameras and display screens~\cite{RIFLE}. The following paragraphs will introduce the formation principle of flicker-banding from the perspective of both the smartphone cameras and display screens.

Firstly, from the capture perspective, smartphone cameras usually use the Complementary Metal-Oxide Semiconductor (CMOS) sensors with an electronic rolling shutter~\cite{durini2019high}. CMOS consists of an integrated circuit design style
depending on groups of p-channel
(PMOS) and n-channel (NMOS) metal-oxide-semiconductor field-effect transistors (MOSFETs)~\cite{2024SensorCMOS}. CMOS sensors expose each line of pixels rather than expose the whole entity when taking photos, which means that each line of pixels on the cameras capture the lightness of the display screens not at the same time. As a result, time offset appears when capturing.

However, since the lightness of display screens also changes periodically, sampling at different points in time captures different phases of the screen's brightness waveform. Then from the perspective of display screens, display screens don't emit light continuously but shine with certain frequency. This is a potential conflict in time offset with the mechanism of the smartphone cameras. For instance, LCD screens apply precisely controlled voltage to change the alignment of liquid crystal modules. This change will in turn change the polarization state of the light from the backlight module~\cite{LCDdisplay}. Finally, this light passes the polarizers combined with the layer of the liquid crystal and the amount of light to pass this layer will be selectively blocked or allowed. This process causes the change of lightness and darkness on each pixel, which shows the images we can see on the screen.

Other technology of display matrix, such as the OLED display screens. The basic method for OLED is the Pulse-Width Modulation (PWM), which controls the lightness and darkness of each pixel with certain high frequency~\cite{geffroy2006organic}. Thus, by controlling the time of lightness in one cycle, the average lightness human beings can see is affected. Also, for the LED matrix display, it operates in a multiplexed scanning mode. This means that rather than illuminate all pixels at the same time, rows or columns of pixels are bright at the certain moment with certain frequency. Therefore, we can see that both the display method of screens and capture of the cameras aren't continuous. So we can get the conclusion that flicker-banding occurs when camera and display refresh rates are misaligned.
\section{Simulation pipeline}
In this part, more details about the formulas to add banding to the raw images with moiréing artifacts will be introduced. In this pipeline, five types of banding artifacts are added: linear uniform banding, diamond banding, curve banding, cracked banding and stochastic perturbed banding. Some examples of each type are shown in Figure~\ref{fig:example of pipeline_supp}.
\begin{figure*}[htbp]
    \centering 
    \begin{subfigure}{\textwidth}
        \centering
        \includegraphics[width=1.0\textwidth]{figures/pipeline_supp5_simple_cropped.pdf}
        \caption{Example of Linear Uniform Banding}
        \label{fig:sub5}
    \end{subfigure}
    
    \vspace{0.5cm} 
    
    \begin{subfigure}{\textwidth}
        \centering
        \includegraphics[width=1.0\textwidth]{figures/pipeline_supp3_curve.pdf}
        \caption{Example of Curve Banding}
        \label{fig:sub3}
    \end{subfigure}
    
    \vspace{0.5cm}

    \begin{subfigure}{\textwidth}
        \centering
        \includegraphics[width=1.0\textwidth]{figures/pipeline_supp1_complex.pdf} 
        \caption{Example of Stochastic Perturbed Banding}
        \label{fig:sub1}
    \end{subfigure}
    
    \vspace{0.5cm}
    
     \begin{subfigure}{\textwidth}
        \centering
        \includegraphics[width=1.0\textwidth]{figures/pipeline_supp4_diamond.pdf}
        \caption{Example of Diamond Banding}
        \label{fig:sub4}
    \end{subfigure}
    
    \vspace{0.5cm}
    
    \begin{subfigure}{\textwidth}
        \centering
        \includegraphics[width=1.0\textwidth]{figures/pipeline_supp2_cracked.pdf}
        \caption{Example of Cracked Banding}
        \label{fig:sub2}
    \end{subfigure}
    \caption{Example of results from the simulation pipeline}
    \label{fig:example of pipeline_supp}
\end{figure*}
To process tilted patterns in images, the first step of adding any of these banding is to change the coordinate system. Suppose the width and height of the image is $W$ and $H$, the original coordinate of the pixel is $(x,y)$($x\in[0,W],y\in[0,H]$) and the new coordinate after putting the center of images as the origin of the new system is $(x_c,y_c)$. The relation between the new coordinate and the original one is shown below:
\begin{equation}
\begin{cases}
x_c=x-\frac{W-1}{2}  \\
y_c=y-\frac{H-1}{2}
\end{cases}
\end{equation}
Based on the new coordinate, a local coordinate system that rotates with the object is constructed, which is called 2D rotation transformation mathematically. Suppose the inclination angle of the stripes relative to the vertical direction as $\theta$ and the coordinate after rotation is $(u,v)$. The formula for this rotation is shown below:
\begin{equation}
\begin{bmatrix} u \\ v \end{bmatrix} = 
\begin{bmatrix} \cos\theta & \sin\theta \\ -\sin\theta & \cos\theta \end{bmatrix} 
\begin{bmatrix} x_c \\ y_c \end{bmatrix}
\end{equation}
Thus, the relation can be written as:
\begin{equation}
\begin{cases}
    u = x_c \cdot \cos\theta + y_c \cdot \sin\theta\\
v = -x_c \cdot \sin\theta + y_c \cdot \cos\theta
\end{cases}
\end{equation}
To avoid setting the pixel too dark, we introduce a minimum gain $G_{min}$, which is set to be $0.02$. Set the smooth masking function, which is used to make the edges of banding smoother, as $M(x,y)$, the baseline intensity factor as $D$, which is selected randomly in our pipeline, and the random noise factor of each stripe as $\eta_k$. The gain applied to every pixel $G(x,y)$ can be defined as:
\begin{equation}
    G(x,y) = \max\left( G_{min}, \; 1 - M(x,y) \cdot (1 - D) \cdot \eta_k \right)
\end{equation}
In our pipeline, we use the following equation to calculate the output $I_{out}(x,y)$ from the input image $I_{in}(x,y)$:
\begin{equation}
\label{eq:total}
    I_{out}(x,y) = I_{in}(x,y) \cdot G(x,y)
\end{equation}
The following paragraphs will introduce the corresponding formulas for the variables mentioned above of each type.
%%\newpage
\subsection{Linear Uniform Banding}
\label{sec:Simple}
To generate stripes with period $P$ (period is the result of the addition of stripe width and stripe gap) and phase $\phi$, the stripe index $k$ of the current pixel and its signed distance $d(x,y)$ relative to the center of that stripe need to be calculated. Suppose the width of stripes $w$. The formula to calculate the stripe index $k$ is shown below:
\begin{equation}
k=\operatorname{round}(\frac{v-\phi}{P})
\end{equation}
From the above equation, the ideal stripe center position corresponding to this index $v_c$ can be written as:
\begin{equation}
v_c = k \cdot P + \phi
\end{equation}
The equation below clarifies the current pixel's signed distance $d(x,y)$ relative to the center of the stripe $k$:
\begin{equation}
d(x,y) = |v(x,y) - v_c| - \frac{w}{2}
\end{equation}
If $d(x,y)<0$, this means that the current pixel is in the stripe $k$ and vice versa.

Then to avoid aliasing effect, the Smoothstep function is applied to create a feathered edge. Suppose the feather radius $f$ and the radius after normalization $t$. The formula about $t$ is shown as below:
\begin{equation}
t =\operatorname{clamp}(\frac{d(x,y)+f}{2f},0,1)
\end{equation}
Then the Smoothstep function $S(x,y)$ can be written as $S(x,y)=t^2(3-2t)$. Furthermore, the smooth masking function $M(x,y)$ is defined, representing the occupancy of the banding:
\begin{equation}
    M(x,y)=1-S(x,y)
\end{equation}
Here, $M(x,y)\in[0,1]$, where $1$ means the center of the banding, the darkest and $0$ is the background.

Bringing all the variables back to the equation~\ref{eq:total}, we can get the formula for adding the linear uniform banding.
%%\newpage
\subsection{Curve Banding}
Based on the new coordinate $(u,v)$ obtained in the first step, we introduce a spatial modulation term, an offset function $C(u)$ dependent on $u$, to realize the effect of curve banding. The effective traverse coordinate $v'(u,v)$ can be written as:
\begin{equation}
    v'(u, v) = v - C(u)
\end{equation}
In our pipeline, we realize two kinds of curve modes: quadratic mode and sinusoidal mode. The quadratic mode simulates geometric distortion resembling a bow shape. Let $A$ as the bending amplitude and $L$ as the normalized size. The middle point of pixels in the whole images on the $u$ axis is expressed as $u_{mid}$. The offset function of quadratic mode $C_{quad}(u)$ is shown below:
\begin{equation}
    C_{quad}(u) = \pm A \cdot \left( \frac{u - u_{mid}}{L} \right)^2
\end{equation}
The second mode, the sinusoidal mode, is designed to simulate the wavy interference pattern. Though in our simulation pipeline we don't apply this mode to produce images, but our program can realize this effect. Let $\lambda$ be the wave length and $\phi$ be the initial phase of the curve. The sinusoidal mode $C_{sin}(u)$ can be expressed in the equation below:
\begin{equation}
C_{sin}(u) = A \cdot \sin\left( \frac{2\pi u}{\lambda} + \varphi \right)
\end{equation}
Similar to the stripe index $k$ calculated in the section~\ref{sec:Simple}, suppose the phase of the whole stripe $\Phi_{stripe}$, the stripe index $k$ can be written as:
\begin{equation}
k = \text{round}\left( \frac{v' - \phi_{stripe}}{P} \right)
\end{equation}
Since the center of the stripe is no longer a constant, but a curve $C(u)+const$, the distance from the pixel to the center of the bending stripe $d(x,y)$ is written as:
\begin{equation}
d(x,y) = \left| v' - (k \cdot P + \phi_{stripe}) \right| - \frac{w}{2}
\end{equation}
Also, using the smoothstep function same as the section~\ref{sec:Simple}, we can get the smooth masking function $M(x,y)$:
\begin{equation}
\label{eq:M}
    M(x,y) = 1 - S\left( \text{clamp}\left( \frac{d + f}{2f}, 0, 1 \right) \right)
\end{equation}
Finally, with all the variables calculated above, the output image can be expressed with the formula~\ref{eq:total}.
%%\newpage
\subsection{Stochastic Perturbed Banding}
Stochastic perturbed banding is supposed to have random position, width, shape and edges. Based on the model of curve banding, we add the process of discrete inter-stripe variations and continuous intra-stripe modulation.

Firstly, to realize discrete inter-stripe variations, we introduce two random variables: position jitter $\Delta p_k$ and width jitter $\Delta w_k$, both of which follow uniform distribution. Suppose the spacing and width jitter amplitude respectively as $J_{pos}$ and $J_{width}$ and the original base width as $\bar{w}$. So we can get the modified center of the stripe $v_c$ and base width $w_k$ for the $i^{th}$ stripe:
\begin{equation}
\begin{cases}
    v_c(k) = k \cdot P + \phi + \Delta p_k\\
    w_k = \bar{w} + \Delta w_k
\end{cases}
\end{equation}
\begin{equation*}
    \text{where } \Delta p_k \sim \mathcal{U}(-J_{\text{pos}}, J_{\text{pos}}), \quad
    \Delta w_k \sim \mathcal{U}(-J_{\text{width}}, J_{\text{width}})
\end{equation*}
Secondly, to simulate the slight jitter when using the rolling shutter of smartphone cameras, we introduce the continuous low-frequency modulation. Suppose the width of the stripe at the $u$ position is $w_{l}(u,k)$ and the wiggle amplitude as $A_{wiggle}$. A smooth noise function $\Omega(u)$ is defined:
\begin{equation}
    w_{l}(u, k) = w_k + A_{wiggle} \cdot \Omega(u)
\end{equation}
Then we introduce the independent edge roughness to simulate the fact that edges of stripes may not be smooth. Noise $\zeta_{top}(u)$ and $\zeta_{bot}(u)$are added respectively to the top edge of stripes $E_{top}$ and the bottom edge $E_{bot}$:
\begin{equation}
\begin{cases}
    E_{top} = v_c(k) + \frac{w_{l}(u, k)}{2} + \sigma_{edge} \cdot \zeta_{top}(u)\\
    E_{bot} = v_c(k) - \frac{w_{l}(u, k)}{2} + \sigma_{edge} \cdot \zeta_{bot}(u)
\end{cases}
\end{equation}
The minimum distance $d_{complex}$ from the pixel $v'$ to the edges are defined as:
\begin{equation}
    d_{complex}(x,y) = -\min\left( E_{top} - v', \; v'- E_{bot} \right)
\end{equation}
Replacing the $d$ in the equation~\ref{eq:M} with the $d_{complex}$, we can get the smooth masking function $M(x,y)$ for the stochastic perturbed banding. Taking these variables back into the equation~\ref{eq:total}, we can finally get the formula for adding the stochastic perturbed banding.
%%\newpage
\subsection{Diamond Banding}
Diamond banding is defined as a 2D pattern rather than a linear uniform stripe, which is L1 norm mathematically. Rather than only consider the $v$ axis, both the stripe index $k_u$ and $k_v$ is considered on the $u$ and $v$ axis. Suppose the period on the $u$ and $v$ axis respectively as $P_u$ and $P_v$ and the center of the $u$ and $v$ axis as $u_c$ and $v_c$. It's easy to get $k_v = \text{round}\left( \frac{v - \phi}{P_v} \right) $ and $k_u = \text{floor}\left( \frac{u}{P_u} \right)$. The equation of the center of the $u$ and $v$ axis as $u_c$ and $v_c$ can be obtained:
\begin{equation}
\begin{cases}
    \quad v_c = k_v \cdot P_v + \phi\\

    \quad u_c = k_u \cdot P_u + \frac{P_u}{2}
    \end{cases}
\end{equation}
It' easy to get the coordinate relative to the center of the diamond $(\delta_u, \delta_v)$:$\delta_u=u-u_c$ and $\delta_v=v-v_c$. Suppose $w$ as the biggest width of the stripes and $\alpha$ as the shear slope, which is determined by the ratio of the height and width of the diamond. So we can get the boundary condition for a pixel to lie inside a diamond:
\begin{equation}
    |\delta_v| + \alpha \cdot |\delta_u| \le \frac{w}{2}
\end{equation}
From the formula above, we can define the distance between the pixel and the boundary of the diamond $d_{diamond}$:
\begin{equation}
    d_{diamond}=(|\delta_v| + \alpha \cdot |\delta_u|)- \frac{w}{2}
\end{equation}
If $d_{diamond}<0$, the pixel is in the diamond and vice versa.

Similar to the model mentioned in the section~\ref{sec:Simple}, the smooth masking function $M(x,y)$ can be written as:
\begin{equation}
    M(x,y) = 1 - S\left( \text{clamp}\left( \frac{d_{diamond} + f}{2f}, 0, 1 \right) \right)
\end{equation}
With all these variables mentioned above, the eqaution~\ref{eq:total} can be written into the form of producing the diamond banding.
%%\newpage
\subsection{Cracked Banding}
The cracked banding is a kind of pattern with the central area continuous and small cracks on the sides. Firstly, we need to define the body of the banding. Set the center keep ratio as $R_{keep}\in(0,1)$ and the half width of the central area as $w_{core}=\frac{w}{2}\cdot R_{keep}$. Suppose the center of the banding as $v_c$ and feathered smoothstep function as $S(\cdot)$. So the smooth masking function of the core area $M_{core}(x,y)$ can be defined as:
\begin{equation}
M_{core} = 1 - S(|v - v_c| - w_{core})
\end{equation}
Secondly, on both sides of the center, we generate $N$ stripes of small parallel crack patterns. For the $i^{th}$ stripe, the distance from the crack center to the stripe main center $v_c$ is set as $\delta_i$, the basic width as $\bar{w}_i$, the dither intensity as $\gamma$ and the dynamic width as $w_i(u)$. To simulate the natural irregularity, random noise $J(u)$ is introduced and the equation can be written as below:
\begin{equation}
    w_i(u) = \bar{w}_i \cdot (1 + \gamma \cdot J(u))
\end{equation}
Then the distance between the pixel and the center of the $i^{th}$ crack can be written as:
\begin{equation}
    d_{i}(x,y) = |v - (v_c + \delta_i)| - \frac{w_i(u)}{2}
\end{equation}
Moreover, to create a discontinuous crack effect, longitudinal breaks are added. We introduce a binary break mask $B_i(u)$:
\begin{equation}
    B_i(u) = \begin{cases} 
0, & \text{if } u \in \text{Break Regions} \\
1, & \text{otherwise}
\end{cases}
\end{equation}
From the equation above, we can get the smoothing mask function $M_{crack, i}(x,y)$ for the $i^{th}$ crack:
\begin{equation}
    M_{crack, i}(x,y) = M_{raw, i}(x,y) \cdot B_i(u)
\end{equation}
Finally, the smoothing mask function $M_{final}$ of the whole crack banding can be written as:
\begin{equation}
    M_{final} = \max\left( M_{core}, \; \max_{i=1}^{N} \{ M_{crack, i} \} \right)
\end{equation}
With all the variables above, it's easy to get the formula for producing cracked banding from the equation~\ref{eq:total}.

\section{Additional Visual Comparison}
In this section, additional visual comparison is presented with flicker-banding and moiré images(LQ), clean images(GT) and other compared methods on the \textbf{MIRAGE} testing dataset in Figure~\ref{fig:supp visual comparison1}--\ref{fig:supp visual comparison3}.
\begin{figure*}[t]
\centering

% ===================== Row 1 =====================
\begin{minipage}[t]{0.19\textwidth}
    \centering
    \includegraphics[width=\linewidth]{figures/supp_visual/GT/GT_60.jpg}\\
    \footnotesize GT
\end{minipage}
\hfill
\begin{minipage}[t]{0.19\textwidth}
    \centering
    \includegraphics[angle=180,origin=c,width=\linewidth]{figures/supp_visual/LQ/LQ_60.jpg}\\
    \footnotesize LQ
\end{minipage}
\hfill
\begin{minipage}[t]{0.19\textwidth}
    \centering
    \includegraphics[angle=180,origin=c,width=\linewidth]{figures/supp_visual/ESDNet/ESDNet_60.png}\\
    \footnotesize ESDNet
\end{minipage}
\hfill
\begin{minipage}[t]{0.19\textwidth}
    \centering
    \includegraphics[angle=180,origin=c,width=\linewidth]{figures/supp_visual/NeRD-Rain/NeRD-Rain_60.png}\\
    \footnotesize NeRD-Rain
\end{minipage}
\hfill
\begin{minipage}[t]{0.19\textwidth}
    \centering
    \includegraphics[angle=180,origin=c,width=\linewidth]{figures/supp_visual/MAT/MAT_60.png}\\
    \footnotesize MAT
\end{minipage}
\vspace{1mm}
% ===================== Row 2 =====================
\begin{minipage}[t]{0.19\textwidth}
    \centering
    \includegraphics[angle=180,origin=c,width=\linewidth]{figures/supp_visual/ResShift/ResShift_60.png}\\
    \footnotesize ResShift
\end{minipage}
\hfill
\begin{minipage}[t]{0.19\textwidth}
    \centering
    \includegraphics[angle=180,origin=c,width=\linewidth]{figures/supp_visual/PiSA-SR/PiSA-SR_60.png}\\
    \footnotesize PiSA-SR
\end{minipage}
\hfill
\begin{minipage}[t]{0.19\textwidth}
    \centering
    \includegraphics[angle=180,origin=c,width=\linewidth]{figures/supp_visual/InvSR/InvSR_60.png}\\
    \footnotesize InvSR
\end{minipage}
\hfill
\begin{minipage}[t]{0.19\textwidth}
    \centering
    \includegraphics[angle=180,origin=c,width=\linewidth]{figures/supp_visual/RIFLE/RIFLE-60.png}\\
    \footnotesize RIFLE
\end{minipage}
\hfill
\begin{minipage}[t]{0.19\textwidth}
    \centering
    \includegraphics[angle=180,origin=c,width=\linewidth]{figures/supp_visual/CLEAR/CLEAR_60.jpg}\\
    \footnotesize CLEAR
\end{minipage}

\begin{minipage}[t]{0.19\textwidth}
    \centering
    \includegraphics[width=\linewidth]{figures/supp_visual/GT/GT_383.png}\\
    \footnotesize GT
\end{minipage}
\hfill
\begin{minipage}[t]{0.19\textwidth}
    \centering
    \includegraphics[width=\linewidth]{figures/supp_visual/LQ/LQ_383.png}\\
    \footnotesize LQ
\end{minipage}
\hfill
\begin{minipage}[t]{0.19\textwidth}
    \centering
    \includegraphics[width=\linewidth]{figures/supp_visual/ESDNet/ESDNet_383.png}\\
    \footnotesize ESDNet
\end{minipage}
\hfill
\begin{minipage}[t]{0.19\textwidth}
    \centering
    \includegraphics[width=\linewidth]{figures/supp_visual/NeRD-Rain/NeRD_Rain_383.png}\\
    \footnotesize NeRD-Rain
\end{minipage}
\hfill
\begin{minipage}[t]{0.19\textwidth}
    \centering
    \includegraphics[width=\linewidth]{figures/supp_visual/MAT/MAT_383.png}\\
    \footnotesize MAT
\end{minipage}
% \vspace{-2mm}
% ===================== Row 2 =====================
\begin{minipage}[t]{0.19\textwidth}
    \centering
    \includegraphics[width=\linewidth]{figures/supp_visual/ResShift/ResShift_383.png}\\
    \footnotesize ResShift
\end{minipage}
\hfill
\begin{minipage}[t]{0.19\textwidth}
    \centering
    \includegraphics[width=\linewidth]{figures/supp_visual/PiSA-SR/PiSA-SR_383.png}\\
    \footnotesize PiSA-SR
\end{minipage}
\hfill
\begin{minipage}[t]{0.19\textwidth}
    \centering
    \includegraphics[width=\linewidth]{figures/supp_visual/InvSR/InvSR_383.png}\\
    \footnotesize InvSR
\end{minipage}
\hfill
\begin{minipage}[t]{0.19\textwidth}
    \centering
    \includegraphics[width=\linewidth]{figures/supp_visual/RIFLE/RIFLE_383.png}\\
    \footnotesize RIFLE
\end{minipage}
\hfill
\begin{minipage}[t]{0.19\textwidth}
    \centering
    \includegraphics[width=\linewidth]{figures/supp_visual/CLEAR/CLEAR_383.png}\\
    \footnotesize CLEAR
\end{minipage}
%Third picture
\begin{minipage}[t]{0.19\textwidth}
    \centering
    \includegraphics[width=\linewidth]{figures/supp_visual/GT/GT_418.png}\\
    \footnotesize GT
\end{minipage}
\hfill
\begin{minipage}[t]{0.19\textwidth}
    \centering
    \includegraphics[width=\linewidth]{figures/supp_visual/LQ/LQ_418.png}\\
    \footnotesize LQ
\end{minipage}
\hfill
\begin{minipage}[t]{0.19\textwidth}
    \centering
    \includegraphics[width=\linewidth]{figures/supp_visual/ESDNet/ESDNet_418.png}\\
    \footnotesize ESDNet
\end{minipage}
\hfill
\begin{minipage}[t]{0.19\textwidth}
    \centering
    \includegraphics[width=\linewidth]{figures/supp_visual/NeRD-Rain/NeRD-Rain_418.png}\\
    \footnotesize NeRD-Rain
\end{minipage}
\hfill
\begin{minipage}[t]{0.19\textwidth}
    \centering
    \includegraphics[width=\linewidth]{figures/supp_visual/MAT/MAT_418.png}\\
    \footnotesize MAT
\end{minipage}
% \vspace{-2mm}
% ===================== Row 2 =====================
\begin{minipage}[t]{0.19\textwidth}
    \centering
    \includegraphics[width=\linewidth]{figures/supp_visual/ResShift/ResShift_418.png}\\
    \footnotesize ResShift
\end{minipage}
\hfill
\begin{minipage}[t]{0.19\textwidth}
    \centering
    \includegraphics[width=\linewidth]{figures/supp_visual/PiSA-SR/PiSA-SR_418.png}\\
    \footnotesize PiSA-SR
\end{minipage}
\hfill
\begin{minipage}[t]{0.19\textwidth}
    \centering
    \includegraphics[width=\linewidth]{figures/supp_visual/InvSR/InvSR_418.png}\\
    \footnotesize InvSR
\end{minipage}
\hfill
\begin{minipage}[t]{0.19\textwidth}
    \centering
    \includegraphics[width=\linewidth]{figures/supp_visual/RIFLE/RIFLE_418.png}\\
    \footnotesize RIFLE
\end{minipage}
\hfill
\begin{minipage}[t]{0.19\textwidth}
    \centering
    \includegraphics[width=\linewidth]{figures/supp_visual/CLEAR/CLEAR_418.png}\\
    \footnotesize CLEAR
\end{minipage}
\vspace{-2mm}
\caption{Visual comparison with flicker-banding \& moiré images (LQ), clean images (GT), and other compared methods on the MIRAGE testing dataset. Compared methods are retrained with MIRAGE's training dataset. CLEAR gains great advantages over other methods.}
\label{fig:supp visual comparison1}
\vspace{-6mm}
\end{figure*}

\begin{figure*}[t]
\centering

% ===================== Row 1 =====================
\begin{minipage}[t]{0.19\textwidth}
    \centering
    \includegraphics[width=\linewidth]{figures/supp_visual/GT/GT_1988.png}\\
    \footnotesize GT
\end{minipage}
\hfill
\begin{minipage}[t]{0.19\textwidth}
    \centering
    \includegraphics[width=\linewidth]{figures/supp_visual/LQ/LQ_1988.png}\\
    \footnotesize LQ
\end{minipage}
\hfill
\begin{minipage}[t]{0.19\textwidth}
    \centering
    \includegraphics[width=\linewidth]{figures/supp_visual/ESDNet/ESDNet_1988.png}\\
    \footnotesize ESDNet
\end{minipage}
\hfill
\begin{minipage}[t]{0.19\textwidth}
    \centering
    \includegraphics[width=\linewidth]{figures/supp_visual/NeRD-Rain/NeRD-Rain_1988.png}\\
    \footnotesize NeRD-Rain
\end{minipage}
\hfill
\begin{minipage}[t]{0.19\textwidth}
    \centering
    \includegraphics[width=\linewidth]{figures/supp_visual/MAT/MAT_1988.png}\\
    \footnotesize MAT
\end{minipage}
\vspace{1mm}
% ===================== Row 2 =====================
\begin{minipage}[t]{0.19\textwidth}
    \centering
    \includegraphics[width=\linewidth]{figures/supp_visual/ResShift/ResShift_1988.png}\\
    \footnotesize ResShift
\end{minipage}
\hfill
\begin{minipage}[t]{0.19\textwidth}
    \centering
    \includegraphics[width=\linewidth]{figures/supp_visual/PiSA-SR/PiSA-SR_1988.png}\\
    \footnotesize PiSA-SR
\end{minipage}
\hfill
\begin{minipage}[t]{0.19\textwidth}
    \centering
    \includegraphics[width=\linewidth]{figures/supp_visual/InvSR/InvSR_1988.png}\\
    \footnotesize InvSR
\end{minipage}
\hfill
\begin{minipage}[t]{0.19\textwidth}
    \centering
    \includegraphics[width=\linewidth]{figures/supp_visual/RIFLE/RIFLE_1988.png}\\
    \footnotesize RIFLE
\end{minipage}
\hfill
\begin{minipage}[t]{0.19\textwidth}
    \centering
    \includegraphics[width=\linewidth]{figures/supp_visual/CLEAR/CLEAR_1988.png}\\
    \footnotesize CLEAR
\end{minipage}

\begin{minipage}[t]{0.19\textwidth}
    \centering
    \includegraphics[width=\linewidth]{figures/visual/selected_images/GT/001938.png}\\
    \footnotesize GT
\end{minipage}
\hfill
\begin{minipage}[t]{0.19\textwidth}
    \centering
    \includegraphics[width=\linewidth]{figures/visual/selected_images/LQ/001938.png}\\
    \footnotesize LQ
\end{minipage}
\hfill
\begin{minipage}[t]{0.19\textwidth}
    \centering
    \includegraphics[width=\linewidth]{figures/visual/selected_images/ESDNet/001938.png}\\
    \footnotesize ESDNet
\end{minipage}
\hfill
\begin{minipage}[t]{0.19\textwidth}
    \centering
    \includegraphics[width=\linewidth]{figures/visual/selected_images/NeRD-Rain/001938.png}\\
    \footnotesize NeRD-Rain
\end{minipage}
\hfill
\begin{minipage}[t]{0.19\textwidth}
    \centering
    \includegraphics[width=\linewidth]{figures/visual/selected_images/MAT/001938.png}\\
    \footnotesize MAT
\end{minipage}
% \vspace{-2mm}
% ===================== Row 2 =====================
\begin{minipage}[t]{0.19\textwidth}
    \centering
    \includegraphics[width=\linewidth]{figures/visual/selected_images/ResShift/001938.png}\\
    \footnotesize ResShift
\end{minipage}
\hfill
\begin{minipage}[t]{0.19\textwidth}
    \centering
    \includegraphics[width=\linewidth]{figures/visual/selected_images/PiSA-SR/001938.png}\\
    \footnotesize PiSA-SR
\end{minipage}
\hfill
\begin{minipage}[t]{0.19\textwidth}
    \centering
    \includegraphics[width=\linewidth]{figures/visual/selected_images/InvSR/001938.png}\\
    \footnotesize InvSR
\end{minipage}
\hfill
\begin{minipage}[t]{0.19\textwidth}
    \centering
    \includegraphics[width=\linewidth]{figures/visual/selected_images/RIFLE/001938.png}\\
    \footnotesize RIFLE
\end{minipage}
\hfill
\begin{minipage}[t]{0.19\textwidth}
    \centering
    \includegraphics[width=\linewidth]{figures/visual/selected_images/CLEAR/001938.png}\\
    \footnotesize CLEAR
\end{minipage}
%Third picture
\begin{minipage}[t]{0.19\textwidth}
    \centering
    \includegraphics[width=\linewidth]{figures/visual/selected_images/GT/001844.png}\\
    \footnotesize GT
\end{minipage}
\hfill
\begin{minipage}[t]{0.19\textwidth}
    \centering
    \includegraphics[width=\linewidth]{figures/visual/selected_images/LQ/001844.png}\\
    \footnotesize LQ
\end{minipage}
\hfill
\begin{minipage}[t]{0.19\textwidth}
    \centering
    \includegraphics[width=\linewidth]{figures/visual/selected_images/ESDNet/001844.png}\\
    \footnotesize ESDNet
\end{minipage}
\hfill
\begin{minipage}[t]{0.19\textwidth}
    \centering
    \includegraphics[width=\linewidth]{figures/visual/selected_images/NeRD-Rain/001844.png}\\
    \footnotesize NeRD-Rain
\end{minipage}
\hfill
\begin{minipage}[t]{0.19\textwidth}
    \centering
    \includegraphics[width=\linewidth]{figures/visual/selected_images/MAT/001844.png}\\
    \footnotesize MAT
\end{minipage}
% \vspace{-2mm}
% ===================== Row 2 =====================
\begin{minipage}[t]{0.19\textwidth}
    \centering
    \includegraphics[width=\linewidth]{figures/visual/selected_images/ResShift/001844.png}\\
    \footnotesize ResShift
\end{minipage}
\hfill
\begin{minipage}[t]{0.19\textwidth}
    \centering
    \includegraphics[width=\linewidth]{figures/visual/selected_images/PiSA-SR/001844.png}\\
    \footnotesize PiSA-SR
\end{minipage}
\hfill
\begin{minipage}[t]{0.19\textwidth}
    \centering
    \includegraphics[width=\linewidth]{figures/visual/selected_images/InvSR/001844.png}\\
    \footnotesize InvSR
\end{minipage}
\hfill
\begin{minipage}[t]{0.19\textwidth}
    \centering
    \includegraphics[width=\linewidth]{figures/visual/selected_images/RIFLE/001844.png}\\
    \footnotesize RIFLE
\end{minipage}
\hfill
\begin{minipage}[t]{0.19\textwidth}
    \centering
    \includegraphics[width=\linewidth]{figures/visual/selected_images/CLEAR/001844.png}\\
    \footnotesize CLEAR
\end{minipage}
\vspace{-2mm}
\caption{Visual comparison with flicker-banding \& moiré images (LQ), clean images (GT), and other compared methods on the MIRAGE testing dataset. Compared methods are retrained with MIRAGE's training dataset. CLEAR gains great advantages over other methods.}
\label{fig:supp visual comparison2}
\vspace{-6mm}
\end{figure*}

\begin{figure*}[t]
\centering

% ===================== Row 1 =====================
\begin{minipage}[t]{0.19\textwidth}
    \centering
    \includegraphics[width=\linewidth]{figures/supp_visual/GT/GT_484.png}\\
    \footnotesize GT
\end{minipage}
\hfill
\begin{minipage}[t]{0.19\textwidth}
    \centering
    \includegraphics[width=\linewidth]{figures/supp_visual/LQ/LQ_484.png}\\
    \footnotesize LQ
\end{minipage}
\hfill
\begin{minipage}[t]{0.19\textwidth}
    \centering
    \includegraphics[width=\linewidth]{figures/supp_visual/ESDNet/ESDNet_484.png}\\
    \footnotesize ESDNet
\end{minipage}
\hfill
\begin{minipage}[t]{0.19\textwidth}
    \centering
    \includegraphics[width=\linewidth]{figures/supp_visual/NeRD-Rain/NeRD-Rain_484.png}\\
    \footnotesize NeRD-Rain
\end{minipage}
\hfill
\begin{minipage}[t]{0.19\textwidth}
    \centering
    \includegraphics[width=\linewidth]{figures/supp_visual/MAT/MAT_484.png}\\
    \footnotesize MAT
\end{minipage}
\vspace{1mm}
% ===================== Row 2 =====================
\begin{minipage}[t]{0.19\textwidth}
    \centering
    \includegraphics[width=\linewidth]{figures/supp_visual/ResShift/ResShift_484.png}\\
    \footnotesize ResShift
\end{minipage}
\hfill
\begin{minipage}[t]{0.19\textwidth}
    \centering
    \includegraphics[width=\linewidth]{figures/supp_visual/PiSA-SR/PiSA-SR_484.png}\\
    \footnotesize PiSA-SR
\end{minipage}
\hfill
\begin{minipage}[t]{0.19\textwidth}
    \centering
    \includegraphics[width=\linewidth]{figures/supp_visual/InvSR/InvSR_484.png}\\
    \footnotesize InvSR
\end{minipage}
\hfill
\begin{minipage}[t]{0.19\textwidth}
    \centering
    \includegraphics[width=\linewidth]{figures/supp_visual/RIFLE/RIFLE_484.png}\\
    \footnotesize RIFLE
\end{minipage}
\hfill
\begin{minipage}[t]{0.19\textwidth}
    \centering
    \includegraphics[width=\linewidth]{figures/supp_visual/CLEAR/CLEAR_484.png}\\
    \footnotesize CLEAR
\end{minipage}

\begin{minipage}[t]{0.19\textwidth}
    \centering
    \includegraphics[width=\linewidth]{figures/supp_visual/GT/GT_490.png}\\
    \footnotesize GT
\end{minipage}
\hfill
\begin{minipage}[t]{0.19\textwidth}
    \centering
    \includegraphics[width=\linewidth]{figures/supp_visual/LQ/LQ_490.png}\\
    \footnotesize LQ
\end{minipage}
\hfill
\begin{minipage}[t]{0.19\textwidth}
    \centering
    \includegraphics[width=\linewidth]{figures/supp_visual/ESDNet/ESDNet_490.png}\\
    \footnotesize ESDNet
\end{minipage}
\hfill
\begin{minipage}[t]{0.19\textwidth}
    \centering
    \includegraphics[width=\linewidth]{figures/supp_visual/NeRD-Rain/NeRD-Rain_490.png}\\
    \footnotesize NeRD-Rain
\end{minipage}
\hfill
\begin{minipage}[t]{0.19\textwidth}
    \centering
    \includegraphics[width=\linewidth]{figures/supp_visual/MAT/MAT_490.png}\\
    \footnotesize MAT
\end{minipage}
% \vspace{-2mm}
% ===================== Row 2 =====================
\begin{minipage}[t]{0.19\textwidth}
    \centering
    \includegraphics[width=\linewidth]{figures/supp_visual/ResShift/ResShift_490.png}\\
    \footnotesize ResShift
\end{minipage}
\hfill
\begin{minipage}[t]{0.19\textwidth}
    \centering
    \includegraphics[width=\linewidth]{figures/supp_visual/PiSA-SR/PiSA-SR_490.png}\\
    \footnotesize PiSA-SR
\end{minipage}
\hfill
\begin{minipage}[t]{0.19\textwidth}
    \centering
    \includegraphics[width=\linewidth]{figures/supp_visual/InvSR/InvSR_490.png}\\
    \footnotesize InvSR
\end{minipage}
\hfill
\begin{minipage}[t]{0.19\textwidth}
    \centering
    \includegraphics[width=\linewidth]{figures/supp_visual/RIFLE/RIFLE_490.png}\\
    \footnotesize RIFLE
\end{minipage}
\hfill
\begin{minipage}[t]{0.19\textwidth}
    \centering
    \includegraphics[width=\linewidth]{figures/supp_visual/CLEAR/CLEAR_490.png}\\
    \footnotesize CLEAR
\end{minipage}
%Third picture
\begin{minipage}[t]{0.19\textwidth}
    \centering
    \includegraphics[width=\linewidth]{figures/supp_visual/GT/GT_501.png}\\
    \footnotesize GT
\end{minipage}
\hfill
\begin{minipage}[t]{0.19\textwidth}
    \centering
    \includegraphics[width=\linewidth]{figures/supp_visual/LQ/LQ_501.png}\\
    \footnotesize LQ
\end{minipage}
\hfill
\begin{minipage}[t]{0.19\textwidth}
    \centering
    \includegraphics[width=\linewidth]{figures/supp_visual/ESDNet/ESDNet_501.png}\\
    \footnotesize ESDNet
\end{minipage}
\hfill
\begin{minipage}[t]{0.19\textwidth}
    \centering
    \includegraphics[width=\linewidth]{figures/supp_visual/NeRD-Rain/NeRD-Rain_501.png}\\
    \footnotesize NeRD-Rain
\end{minipage}
\hfill
\begin{minipage}[t]{0.19\textwidth}
    \centering
    \includegraphics[width=\linewidth]{figures/supp_visual/MAT/MAT_501.png}\\
    \footnotesize MAT
\end{minipage}
% \vspace{-2mm}
% ===================== Row 2 =====================
\begin{minipage}[t]{0.19\textwidth}
    \centering
    \includegraphics[width=\linewidth]{figures/supp_visual/ResShift/ResShift_501.png}\\
    \footnotesize ResShift
\end{minipage}
\hfill
\begin{minipage}[t]{0.19\textwidth}
    \centering
    \includegraphics[width=\linewidth]{figures/supp_visual/PiSA-SR/PiSA-SR_501.png}\\
    \footnotesize PiSA-SR
\end{minipage}
\hfill
\begin{minipage}[t]{0.19\textwidth}
    \centering
    \includegraphics[width=\linewidth]{figures/supp_visual/InvSR/InvSR_501.png}\\
    \footnotesize InvSR
\end{minipage}
\hfill
\begin{minipage}[t]{0.19\textwidth}
    \centering
    \includegraphics[width=\linewidth]{figures/supp_visual/RIFLE/RIFLE_501.png}\\
    \footnotesize RIFLE
\end{minipage}
\hfill
\begin{minipage}[t]{0.19\textwidth}
    \centering
    \includegraphics[width=\linewidth]{figures/supp_visual/CLEAR/CLEAR_501.png}\\
    \footnotesize CLEAR
\end{minipage}
\vspace{-2mm}
\caption{Visual comparison with flicker-banding \& moiré images (LQ), clean images (GT), and other compared methods on the MIRAGE testing dataset. Compared methods are retrained with MIRAGE's training dataset. CLEAR gains great advantages over other methods.}
\label{fig:supp visual comparison3}
\vspace{-6mm}
\end{figure*}
\section{Results for Debanding}
This section will show results of debanding with CLEAR. Visual comparison between CLEAR, flicker-banding images (LQ), clean images (GT) and RIFLE on the MIRAGE testing dataset in Figure~\ref{fig:supp_B}. We can see that CLEAR has a better performance in image debanding.

\begin{figure*}[t]
    \centering
    \begin{minipage}[t]{0.24\textwidth} 
        \centering
        \includegraphics[width=0.95\linewidth]{figures/supp_banding/LQ/LQ_97.png}
        \caption*{\footnotesize LQ}
    \end{minipage}
    \hfill
    \begin{minipage}[t]{0.24\textwidth} 
        \centering
        \includegraphics[width=0.95\linewidth]{figures/supp_banding/GT/GT_97.png}
        \caption*{\footnotesize GT}
    \end{minipage}
    \hfill
    \begin{minipage}[t]{0.24\textwidth} 
        \centering
        \includegraphics[width=0.95\linewidth]{figures/supp_banding/RIFLE/RIFLE_97.png}
        \caption*{\footnotesize RIFLE}
    \end{minipage}
    \hfill
    \begin{minipage}[t]{0.24\textwidth} 
        \centering
        \includegraphics[width=0.95\linewidth]{figures/supp_banding/CLEAR/CLEAR_97.png}
        \caption*{\footnotesize CLEAR}
    \end{minipage}
    
%\vspace{0.2cm}

           \begin{minipage}[t]{0.24\textwidth} 
        \centering
        \includegraphics[width=0.95\linewidth]{figures/supp_banding/LQ/LQ_168.png}
        \caption*{\footnotesize LQ}
    \end{minipage}
    \hfill
    \begin{minipage}[t]{0.24\textwidth} 
        \centering
        \includegraphics[width=0.95\linewidth]{figures/supp_banding/GT/GT_168.png}
        \caption*{\footnotesize GT}
    \end{minipage}
    \hfill
    \begin{minipage}[t]{0.24\textwidth} 
        \centering
        \includegraphics[width=0.95\linewidth]{figures/supp_banding/RIFLE/RIFLE_168.png}
        \caption*{\footnotesize RIFLE}
    \end{minipage}
    \hfill
    \begin{minipage}[t]{0.24\textwidth} 
        \centering
        \includegraphics[width=0.95\linewidth]{figures/supp_banding/CLEAR/CLEAR_168.png}
        \caption*{\footnotesize CLEAR}
    \end{minipage}

 \begin{minipage}[t]{0.24\textwidth} 
        \centering
        \includegraphics[width=0.95\linewidth]{figures/supp_banding/LQ/LQ_203.png}
        \caption*{\footnotesize LQ}
    \end{minipage}
    \hfill
    \begin{minipage}[t]{0.24\textwidth} 
        \centering
        \includegraphics[width=0.95\linewidth]{figures/supp_banding/GT/GT_203.png}
        \caption*{\footnotesize GT}
    \end{minipage}
    \hfill
    \begin{minipage}[t]{0.24\textwidth} 
        \centering
        \includegraphics[width=0.95\linewidth]{figures/supp_banding/RIFLE/RIFLE_203.png}
        \caption*{\footnotesize RIFLE}
    \end{minipage}
    \hfill
    \begin{minipage}[t]{0.24\textwidth} 
        \centering
        \includegraphics[width=0.95\linewidth]{figures/supp_banding/CLEAR/CLEAR_203.png}
        \caption*{\footnotesize CLEAR}
    \end{minipage}

     \begin{minipage}[t]{0.24\textwidth} 
        \centering
        \includegraphics[width=0.95\linewidth]{figures/supp_banding/LQ/LQ_34.png}
        \caption*{\footnotesize LQ}
    \end{minipage}
    \hfill
    \begin{minipage}[t]{0.24\textwidth} 
        \centering
        \includegraphics[width=0.95\linewidth]{figures/supp_banding/GT/GT_34.png}
        \caption*{\footnotesize GT}
    \end{minipage}
    \hfill
    \begin{minipage}[t]{0.24\textwidth} 
        \centering
        \includegraphics[width=0.95\linewidth]{figures/supp_banding/RIFLE/RIFLE_34.png}
        \caption*{\footnotesize RIFLE}
    \end{minipage}
    \hfill
    \begin{minipage}[t]{0.24\textwidth} 
        \centering
        \includegraphics[width=0.95\linewidth]{figures/supp_banding/CLEAR/CLEAR_34.png}
        \caption*{\footnotesize CLEAR}
    \end{minipage}

 \begin{minipage}[t]{0.24\textwidth} 
        \centering
        \includegraphics[width=0.95\linewidth]{figures/supp_banding/LQ/LQ_48.png}
        \caption*{\footnotesize LQ}
    \end{minipage}
    \hfill
    \begin{minipage}[t]{0.24\textwidth} 
        \centering
        \includegraphics[width=0.95\linewidth]{figures/supp_banding/GT/GT_48.png}
        \caption*{\footnotesize GT}
    \end{minipage}
    \hfill
    \begin{minipage}[t]{0.24\textwidth} 
        \centering
        \includegraphics[width=0.95\linewidth]{figures/supp_banding/RIFLE/RIFLE_48.png}
        \caption*{\footnotesize RIFLE}
    \end{minipage}
    \hfill
    \begin{minipage}[t]{0.24\textwidth} 
        \centering
        \includegraphics[width=0.95\linewidth]{figures/supp_banding/CLEAR/CLEAR_48.png}
        \caption*{\footnotesize CLEAR}
    \end{minipage}
    
    \caption{Visual comparison between CLEAR, flicker-banding images (LQ), clean images (GT) and RIFLE on the MIRAGE testing dataset.}
    \label{fig:supp_B}
\end{figure*}

\section{Results for Demoiréing}
This section will represent comparison between CLEAR, moiré images (LQ), clean images (GT) and ESDNet on the MIRAGE testing dataset as shown in Figure~\ref{fig:supp_M}. We can see that CLEAR performs better in image demoiréing.

\begin{figure*}[t]
    \centering
    \begin{minipage}[t]{0.24\textwidth} 
        \centering
        \includegraphics[width=0.95\linewidth]{figures/supp_moire/LQ/LQ_192.png}
        \caption*{\footnotesize LQ}
    \end{minipage}
    \hfill
    \begin{minipage}[t]{0.24\textwidth} 
        \centering
        \includegraphics[width=0.95\linewidth]{figures/supp_moire/GT/GT_192.png}
        \caption*{\footnotesize GT}
    \end{minipage}
    \hfill
    \begin{minipage}[t]{0.24\textwidth} 
        \centering
        \includegraphics[width=0.95\linewidth]{figures/supp_moire/ESDNet/ESDNet_192.png}
        \caption*{\footnotesize ESDNet}
    \end{minipage}
    \hfill
    \begin{minipage}[t]{0.24\textwidth} 
        \centering
        \includegraphics[width=0.95\linewidth]{figures/supp_moire/CLEAR/CLEAR_192.png}
        \caption*{\footnotesize CLEAR}
    \end{minipage}
    
%\vspace{0.2cm}

           \begin{minipage}[t]{0.24\textwidth} 
        \centering
        \includegraphics[width=0.95\linewidth]{figures/supp_moire/LQ/LQ_90.png}
        \caption*{\footnotesize LQ}
    \end{minipage}
    \hfill
    \begin{minipage}[t]{0.24\textwidth} 
        \centering
        \includegraphics[width=0.95\linewidth]{figures/supp_moire/GT/GT_90.png}
        \caption*{\footnotesize GT}
    \end{minipage}
    \hfill
    \begin{minipage}[t]{0.24\textwidth} 
        \centering
        \includegraphics[width=0.95\linewidth]{figures/supp_moire/ESDNet/ESDNet_90.png}
        \caption*{\footnotesize ESDNet}
    \end{minipage}
    \hfill
    \begin{minipage}[t]{0.24\textwidth} 
        \centering
        \includegraphics[width=0.95\linewidth]{figures/supp_moire/CLEAR/CLEAR_90.png}
        \caption*{\footnotesize CLEAR}
    \end{minipage}

 \begin{minipage}[t]{0.24\textwidth} 
        \centering
        \includegraphics[width=0.95\linewidth]{figures/supp_moire/LQ/LQ_58.png}
        \caption*{\footnotesize LQ}
    \end{minipage}
    \hfill
    \begin{minipage}[t]{0.24\textwidth} 
        \centering
        \includegraphics[width=0.95\linewidth]{figures/supp_moire/GT/GT_58.png}
        \caption*{\footnotesize GT}
    \end{minipage}
    \hfill
    \begin{minipage}[t]{0.24\textwidth} 
        \centering
        \includegraphics[width=0.95\linewidth]{figures/supp_moire/ESDNet/ESDNet_58.png}
        \caption*{\footnotesize ESDNet}
    \end{minipage}
    \hfill
    \begin{minipage}[t]{0.24\textwidth} 
        \centering
        \includegraphics[width=0.95\linewidth]{figures/supp_moire/CLEAR/CLEAR_58.png}
        \caption*{\footnotesize CLEAR}
    \end{minipage}

     \begin{minipage}[t]{0.24\textwidth} 
        \centering
        \includegraphics[width=0.95\linewidth]{figures/supp_moire/LQ/LQ_20.png}
        \caption*{\footnotesize LQ}
    \end{minipage}
    \hfill
    \begin{minipage}[t]{0.24\textwidth} 
        \centering
        \includegraphics[width=0.95\linewidth]{figures/supp_moire/GT/GT_20.png}
        \caption*{\footnotesize GT}
    \end{minipage}
    \hfill
    \begin{minipage}[t]{0.24\textwidth} 
        \centering
        \includegraphics[width=0.95\linewidth]{figures/supp_moire/ESDNet/ESDNet_20.png}
        \caption*{\footnotesize ESDNet}
    \end{minipage}
    \hfill
    \begin{minipage}[t]{0.24\textwidth} 
        \centering
        \includegraphics[width=0.95\linewidth]{figures/supp_moire/CLEAR/CLEAR_20.png}
        \caption*{\footnotesize CLEAR}
    \end{minipage}

 \begin{minipage}[t]{0.24\textwidth} 
        \centering
        \includegraphics[width=0.95\linewidth]{figures/supp_moire/LQ/LQ_37.png}
        \caption*{\footnotesize LQ}
    \end{minipage}
    \hfill
    \begin{minipage}[t]{0.24\textwidth} 
        \centering
        \includegraphics[width=0.95\linewidth]{figures/supp_moire/GT/GT_37.png}
        \caption*{\footnotesize GT}
    \end{minipage}
    \hfill
    \begin{minipage}[t]{0.24\textwidth} 
        \centering
        \includegraphics[width=0.95\linewidth]{figures/supp_moire/ESDNet/ESDNet_37.png}
        \caption*{\footnotesize ESDNet}
    \end{minipage}
    \hfill
    \begin{minipage}[t]{0.24\textwidth} 
        \centering
        \includegraphics[width=0.95\linewidth]{figures/supp_moire/CLEAR/CLEAR_37.png}
        \caption*{\footnotesize CLEAR}
    \end{minipage}
    
    \caption{Visual comparison between CLEAR, moiré images (LQ), clean images (GT) and ESDNet on the MIRAGE testing dataset.}
    \label{fig:supp_M}
\end{figure*}

\bibliography{example_paper}
\bibliographystyle{icml2026}

%%%%%%%%%%%%%%%%%%%%%%%%%%%%%%%%%%%%%%%%%%%%%%%%%%%%%%%%%%%%%%%%%%%%%%%%%%%%%%%
%%%%%%%%%%%%%%%%%%%%%%%%%%%%%%%%%
%%%%%%%%%%%%%%%%%%%%%%%%%%%%%%%%%%%%%%%%%%%%%%%%%%%%%%%%%%%%%%%%%%%%%%%%%%%%%%%
%%%%%%%%%%%%%%%%%%%%%%%%%%%%%%%%%%%%%%%%%%%%%%%%%%%%%%%%%%%%%%%%%%%%%%%%%%%%%%%

\end{document}
